# Supplementary material for: Pano360: Perspective to Panoramic Vision with Geometric Consistency
Source: arXiv:2603.12013 source file (2026-03-12)
Supplement: Supplementary file 1 [file X_suppl.tex]

\clearpage
\setcounter{page}{1}
% \maketitlesupplementary

\appendix

\noindent{\Large \textbf{Appendix}}
\vspace{0.6cm}

\noindent In this Appendix, we provide the following:
\begin{itemize}
    \item Detail the supported projection formats in~\cref{sec:projection formats}.
    \item Comprehensive implementation details for the local mesh warp in~\cref{sec:Mesh_warp}.
    \item The implementation details of bundle adjustment and discussions in~\cref{sec:BA}.
    \item Additional training details in~\cref{sec:train_detail}.
    \item Explanation of seam mask detection in~\cref{sec:seam_mask_explan}
\end{itemize}

\section{Projection Formats}
\label{sec:projection formats}

Our method leverages camera parameters rather than homography, enabling support for various projection formats. We first map the camera parameters to their corresponding yaw $\phi\in [-\pi, \pi]$ and pitch $\theta\in [-\frac{\pi}{2}, \frac{\pi}{2}]$ angles. These angles are then utilized to perform a non-linear mapping. Following the detailed illustration in~\cite{lin2025one}, we introduce several common projection formats in panoramic vision below.

\noindent\textbf{Spherical Projection.} A 360$^{\circ}$ camera is modeled as a pinhole at the center of a unit sphere. All points from the 3D environment are projected onto this sphere. First, a 3D point $\mathbf{P} = [x,y,z]^{\mathrm{T}}$ is converted to spherical coordinates $(\rho, \theta, \phi)$. Here, $\rho$ is the radial distance $\sqrt{x^2 + y^2 + z^2}$, $\theta$ is the polar angle, and $\phi$ is the azimuthal angle. The point is then mapped to the unit sphere by normalizing its radius. This creates a directional unit vector $\mathbf{p} = (\sin\theta\cos\phi, \sin\theta\sin\phi, \cos\theta)$. This method provides a distortion-free representation of all viewing directions.

\noindent\textbf{Equirectangular Projection (ERP).} ERP is the most common format for 360$^{\circ}$ panoramas. It unwraps the spherical surface into a 2D grid. This format directly maps spherical coordinates $(\phi, \theta)$ to image coordinates. The longitude $\phi$ corresponds to the horizontal axis, and the latitude $\theta$ corresponds to the vertical axis. This mapping is simple, like a world map, and very efficient for processing. However, it causes severe geometric distortion at the top and bottom of the image (the poles).

\noindent\textbf{Cubemap Projection (CMP).} CMP is an alternative to ERP that reduces image distortion. It projects the spherical scene onto the six inner faces of a virtual cube. Each face covers a $90^{\circ} \times 90^{\circ}$ field of view. A 3D point $\mathbf{p} = [x',y',z']^{\mathrm{T}}$ on the sphere is mapped to one of the six faces using perspective projection. This is based on its largest coordinate component. For example, for a point mapping to the front face, the 2D coordinates are calculated as $u = x'/|z'|$ and $v = y'/|z'|$. This segmented representation has much less distortion.

\noindent\textbf{Tangent Projection (TP).} To use traditional perspective-based models on spherical data, tangent projection renders the image as a series of local planar grids. These grids are generated by projecting the sphere onto planes tangent to a polyhedron (like an icosahedron). Each patch is formed by a gnomonic projection. A point on the sphere at $(\theta, \phi)$ is mapped to a plane centered at $(\theta_c, \phi_c)$. The resulting planar coordinates $(u_t, v_t)$ are given by:
\begin{align*}
    u_t &= \frac{\cos\phi \sin(\theta - \theta_c)}{\cos c}, \\
    v_t &= \frac{\cos\phi_c \sin\phi - \sin\phi_c \cos\phi \cos(\theta - \theta_c)}{\cos c},
\end{align*}
where $c$ is the central angle between the point and the plane's center. This approach preserves local geometry and reduces distortion.

\noindent\textbf{Polyhedron Projection (PP).} Polyhedron projection approximates the sphere with a subdivided polyhedron, usually an icosahedron. The faces of the polyhedron are recursively divided into smaller triangular facets. For an icosahedron starting at level $l=0$, each new level of subdivision results in $20 \times 4^l$ total faces. This hierarchical subdivision creates a finer approximation of the sphere, leading to more uniform sampling and less distortion.

\noindent\textbf{Panini Projection.} The Panini projection addresses extreme distortions in wide-angle images. It keeps vertical and radial lines straight while applying a non-linear compression horizontally. This maintains a strong perspective feel at the center and avoids excessive stretching at the periphery. The mapping is controlled by a parameter $d \geq 0$:
\[ S = \frac{d+1}{d + \cos\phi}, \quad h = S \cdot \sin\phi, \quad v = S \cdot \tan\theta. \]
The parameter $d$ allows a smooth trade-off between different effects, from a rectilinear projection ($d=0$) to an orthographic-like projection ($d \to \infty$).

\noindent\textbf{360$^{\circ}$ Little Planet Projection.} This projection is usually generated from an ERP image. It transforms the panorama into a circular artwork that looks like a small planet. The effect is achieved using stereographic projection. The entire spherical scene is projected onto a plane from a single point, usually the zenith (top pole). This places the nadir (bottom pole) at the image center and stretches the zenith to the outer boundary. A point $(x, y, z)$ on the sphere is mapped to $(X, Y) = \left(\frac{x}{1-z}, \frac{y}{1-z}\right)$. This projection preserves local angles and shapes but introduces significant area distortion. This distortion creates the unique "little planet" effect, making it popular for artistic purposes.

\noindent\textbf{Other projections.} In addition to the widely-used projection formats mentioned above, our method also supports the conventional projections, including planar, cylindrical, and fisheye. For any projection method, as long as the camera parameters of each image are known, the mapping can be performed. Each scene has its suitable projection format.

\begin{figure*}[t] % [t] 建议将图片置于页面的顶部 (top)
    \centering
    
    \includegraphics[width=1.0\textwidth]{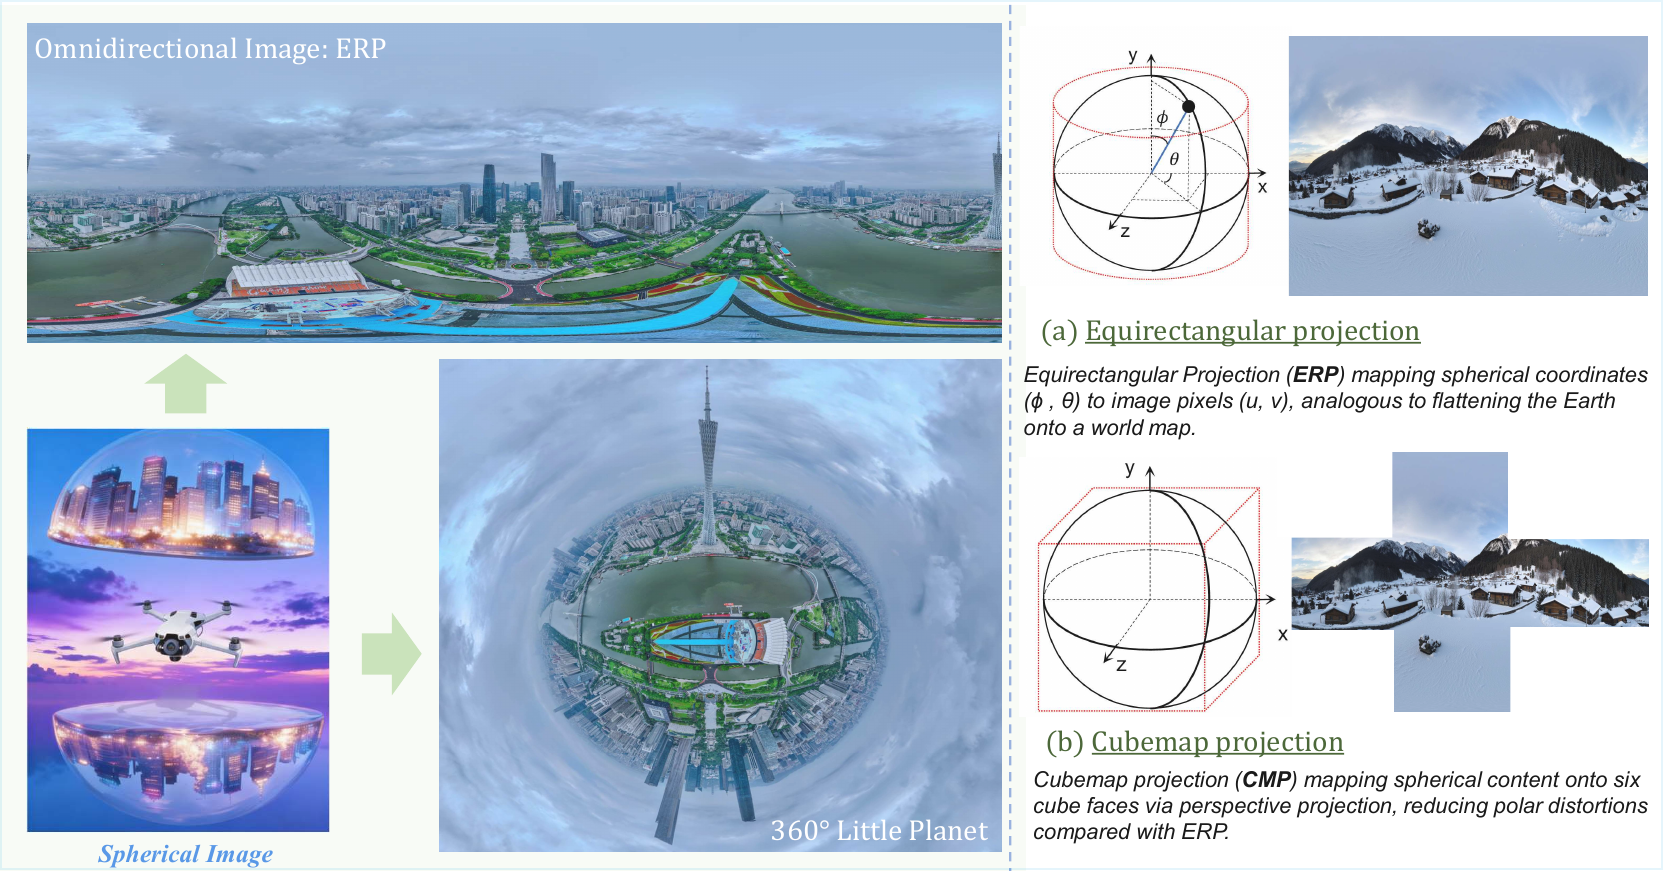}
    
    \caption{From spherical image to panoramic ERP and 360° little planet panorama. ERP preserves a complete field of view compared to perspective images. It maps image each pixels to the spherical coordinates.}
    \label{fig:ERP360}
\end{figure*}

\section{Mesh Warp}
\label{sec:Mesh_warp}

A typical challenge remains in scenes with significant parallax or depth variation, typically addressed by partitioning the image into grids and estimating a local homography for each grid. However, as the grid adjustment is non-differentiable, this technique is not necessary component of our method and dataset with large FoV. In fact, it is not required — as it still aims to achieve visually seamless alignment between pairwise images, at the cost of breaking the geometric structure. Moreover, local mesh adjustments are difficult to employ in practical applications, as the primary focus is the global alignment of the scene. In practice, optical flow is more commonly used to compensate for parallax.

To address scenes with significant parallax or depth variations, similar to APAP~\cite{zaragoza2013projective}, it independently estimates a homography for each grid to eliminate parallax through mesh adjustment. We propose a refined mesh warp method. This approach aims to jointly optimize homographies for regions sharing consistent disparity, thereby achieving seamless alignment between image pairs while preserving the original geometric structure. The process begins by partitioning the overlapping regions of a reference frame ($I_a$) and a target frame ($I_b$). Specifically, $I_a$ is divided into $m$ horizontal strips $\{B_i\}_{i=1}^m$, and $I_b$ is divided into an $m \times n$ grid of blocks $\{G_{i,j}\}_{i=1,j=1}^{m,n}$. To find the optimal correspondence, we compute the Normalized Cross-Correlation (NCC) between each reference block $B_i$ and each candidate block $G_{i,j}$:
\begin{equation}
C(B_i, G_{i,j}) = 
\frac{\sum_{x,y} (B_i(x,y) - \mu_{B_i}) (G_{i,j}(x,y) - \mu_{G_{i,j}})}
{\sigma_{B_i} \cdot \sigma_{G_{i,j}}}
\label{eq:ncc}
\end{equation}
where $\mu$ and $\sigma$ represent the mean intensity and standard deviation of the respective blocks. The optimal displacement $\Delta w^*$ is determined by maximizing the NCC score, which yields the initial disparity $d_{i,j}$:
\begin{equation}
d_{i,j} = \arg \max_{\Delta w} \ C(B_i, G_{i,j}(x+\Delta w, y))
\label{eq:init_disp}
\end{equation}

To ensure matching reliability, we compute a confidence score $M_{i,j}$ for each candidate block, integrating cues such as disparity consistency, spatial support, and similarity:
\begin{equation}
M_{i,j} = w_1 \cdot \rho(d_{i,j}, \bar{d}_i) + w_2 \cdot \eta_{i,j} + w_3 \cdot C(B_i, G_{i,j})
\label{eq:confidence}
\end{equation}

Here, $\rho$ measures the consistency between a candidate disparity and the mean disparity of its neighborhood, while $\eta$ represents the effective spatial support. The block with the highest confidence score is selected as the credible match. Subsequently, adjacent rows are grouped into coherent regions $\mathcal{R}_k$ based on disparity consistency, a process governed by a disparity threshold $\tau_d$ to control region smoothness. To further refine local alignment, we apply a bi-directional region expansion originating from high-confidence seed rows. This process iterates until convergence, yielding a refined disparity field $D^*$ that preserves regional smoothness.

Finally, the mesh warp is updated based on the refined disparity field $D^*$. Each vertex $p=(x,y)$ in the mesh is transformed using a local affine model estimated from its corresponding region $\mathcal{R}_i$:
\begin{equation}
p' = \mathcal{A}_i p + t_i
\label{eq:affine}
\end{equation}
where $\mathcal{A}_i$ and $t_i$ represent the local affine matrix and translation vector, respectively. The updated mesh is then reprojected onto the spherical domain via a new mapping function, producing a seamless panoramic image. This coarse-to-fine framework, which integrates block-wise NCC matching, region-consistent filtering, and affine mesh refinement, achieves accurate and robust alignment even under challenging conditions such as textureless regions, dynamic scenes, or multi-depth environments.

\section{Bundle Adjustment}
\label{sec:BA}
Previous research \cite{yang2025advancements} has primarily focused on visually seamless panoramas and rarely considered camera poses. In contrast, we utilize camera parameters for image alignment. Furthermore, we demonstrate that in certain scenarios, incorporating bundle adjustment can further improve alignment accuracy. However, for challenging scenes with weak texture, large parallax, and repetitive patterns, bundle adjustment may lead to optimization failure or a decrease in accuracy due to the absence of reliable feature correspondences. Consequently, the use of bundle adjustment should be adapted to the specific context of the scene.

Different from bundle adjustment as in SfM~\cite{wang2024vggsfm}, it relies on depth maps to optimize 3D scene coordinates and camera parameters. We consider this task as 2D-to-2D coordinates optimization problem. For points $\mathbf{X}_i$ in image $I_i$ and its matched points $\mathbf{X}_j$ in image $I_j$, we aim to minimize the reprojection error of all matched point pairs:

\begin{equation}
\min_{ \{c_k\} } L = \sum_{(i,j) \in \mathcal{M}}\sum_{k \in \mathcal{K}_{ij}} \| \mathbf{X_j} - \Pi_{\mathbf{P_{i \rightarrow j}}} (\mathbf{\mathbf{X_i}}) \|^2
\label{eq:mapping}
\end{equation}

$\mathcal{M}$ denotes the set of all matched camera pairs, and $\mathcal{K}$ denotes the set of feature point correspondences between a camera pair $(i, j)$. $ \{c_k\} $ represents the camera parameters to be optimized, each with 6 degrees of freedom (6-DoF), including focal length , principal point, and rotation. The rotation is parameterized by a 3D angle-axis vector to avoid constraints. For a pinhole camera, the image pair is mapped by a planar homography $\mathbf{H}_{i \rightarrow j} = \mathbf{K}_j \mathbf{R}_j \mathbf{R}_i^{T} \mathbf{K}_i^{-1}$.

To solve this nonlinear least-squares problem, we employ the Levenberg–Marquardt (LM) algorithm to optimize the camera parameters. Assume $J = \frac{\partial \mathbf{r}}{\partial c}$, where $\mathbf{r}$ is the residual vector composed of all reprojection errors from \cref{eq:mapping}. The iterative update is then given by:

\begin{equation} 
(J^T J + \lambda I) \Delta c = J^T \mathbf{r} 
\label{eq:lm} 
\end{equation}

where $I$ is the identity matrix and $\lambda$ is a damping factor. The matrix $J^T J$ is highly sparse, which can be efficiently computed  by symbolic method. The update vector $\Delta c$ is applied to the camera parameters via $ c \leftarrow c - \Delta c$.

\section{Training Details}
\label{sec:train_detail}

We employ a two-stage training strategy. 
In the first stage, the model is trained on low-resolution ($224 \times 224$ pixels) images for expedited convergence. 
In the second stage, it is fine-tuned on high-resolution images, which are resized to a maximum dimension of 518 pixels while the aspect ratio is randomly sampled from [0.33, 1.0].
For both stages, we use the AdamW optimizer with an initial learning rate of $5 \times 10^{-6}$. 
Each stage runs for 30 epochs, with each epoch consisting of 100 iterations. 
We adopt a dynamic batch sizing strategy similar to VGGT, where each batch comprises 2 to 24 consecutive images with sufficient overlap, sampled from a random training scene. 
Standard data augmentation techniques are applied, including Gaussian blur, color jitter, and exposure adjustment. 
To ensure training stability, we apply gradient clipping with a norm of 1.0. 
Our model is not trained from scratch. 
We initialize the weights of the alternating attention module and the camera decoder from a pre-trained VGGT model, keeping the encoder frozen throughout the training process. 
The all training stages are performed on A100 GPUs in less than one day. 

\section{Seam Mask}
\label{sec:seam_mask_explan}
We leverage a multi-feature joint optimization strategy to compute the seamline, which is subsequently accelerated via neural network distillation on DPT-style~\cite{ranftl2021vision} head. This approach considers the pixel content of all images within a single overlap region simultaneously, thereby avoiding the local optimal that can result from pairwise computations. The most critical component is the texture term, which assigns weights to image regions to guide the seamline away from undesirable areas, such as dynamic objects. For instance, in static scenes, the seam should be guided towards complex, high-gradient areas, making it less perceptible to the human eye. In dynamic scenes, however, it must avoid these paths to prevent cutting through moving objects, which would cause severe artifacts. Although this guidance is based on principles of human visual perception, we consider that by integrating these components into our training framework, our method demonstrates significant advantages over traditional pairwise approaches, particularly in dynamic scenes.

\begin{figure*}[t] % [t] 建议将图片置于页面的顶部 (top)
    \centering
    
    \includegraphics[width=1.0\textwidth]{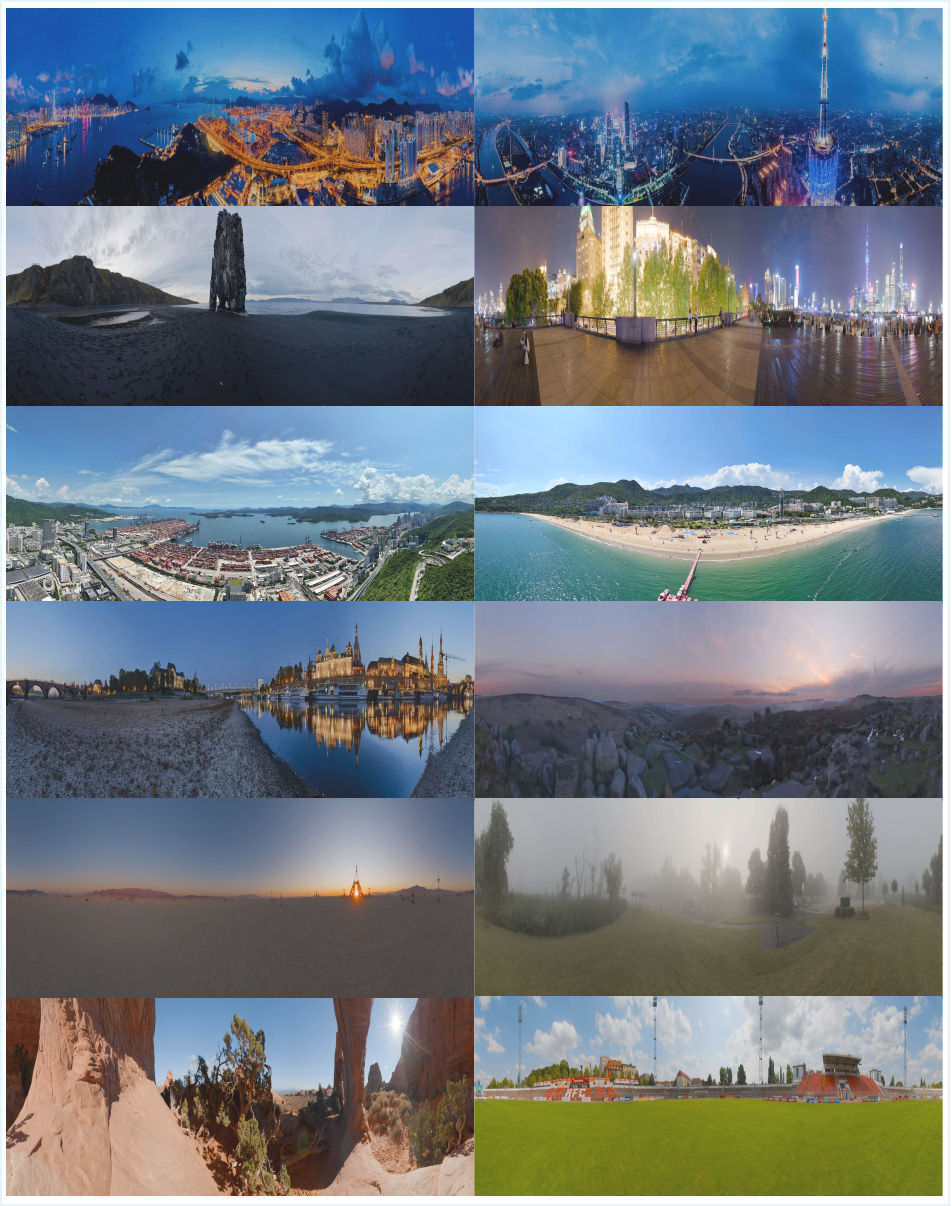}
    
    \caption{More results from our panoramic dataset.}
    \label{fig:MoreResult1}
\end{figure*}

\begin{figure*}[t] % [t] 建议将图片置于页面的顶部 (top)
    \centering
    
    \includegraphics[width=0.8\textwidth]{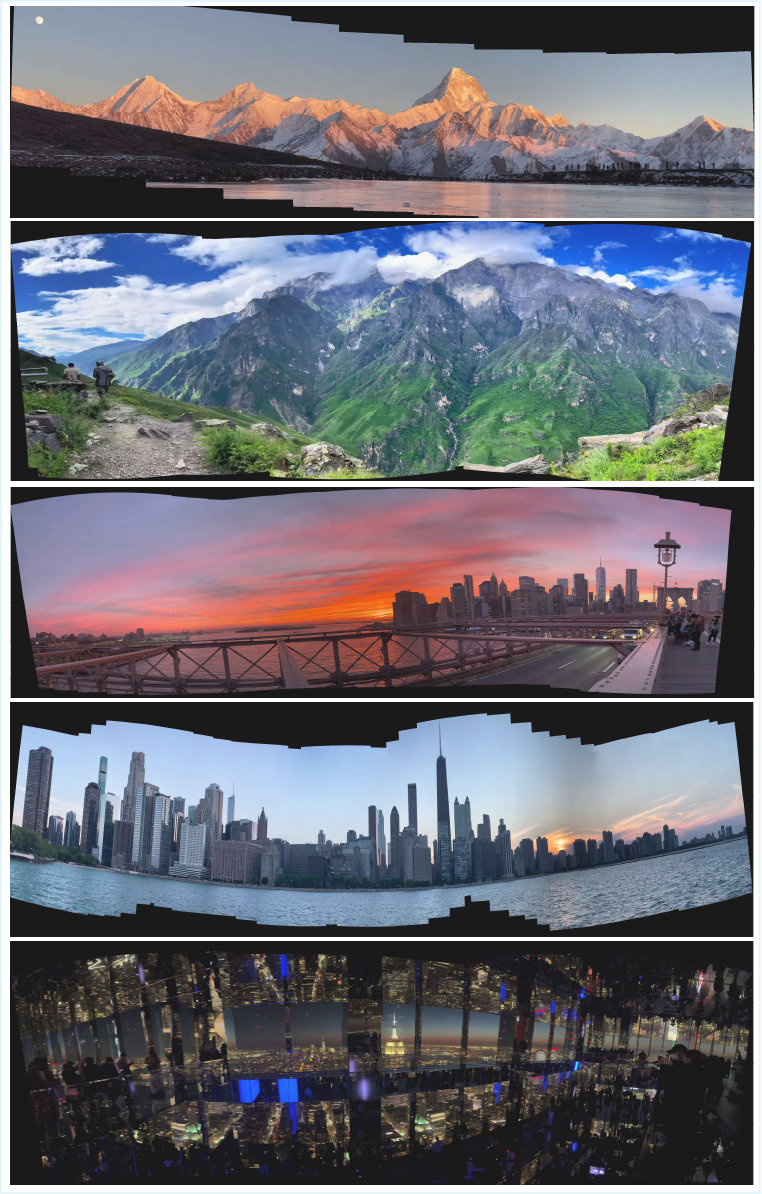}
    
    \caption{More results from in-the-wild dynamic scenes.}
    \label{fig:MoreResult2}
\end{figure*}
